# Supplementary material for: Attribute Based Administration of Role Based Access Control : A Detailed Description
Source: arXiv:1706.03171 source file (2017-07-02)
Supplement: Supplementary file 1 [file appendix.tex]

\appendices
\label{appendix}
\section{Mapping an Example URA97 Instance in AURA}\label{ura97instance}

\noindent
\textbf{An Example URA97 Instance:}\\
\underline{Sets \& Relations:} \\
%\begin{itemize}
-- \U\ = \{\textbf{u\textsubscript1, u\textsubscript2, u\textsubscript3, u\textsubscript4}\}  \\
-- \R\ = \{\textbf{x\textsubscript{1}, x\textsubscript{2}, x\textsubscript{3}, x\textsubscript4, x\textsubscript5, x\textsubscript6}\} \\
-- \AR\ = \{\textbf{ar\textsubscript{1}, ar\textsubscript2}\} \\
-- \UA\ = \{(\textbf{u\textsubscript1, x\textsubscript1}), (\textbf{u\textsubscript1, x\textsubscript2}), (\textbf{u\textsubscript2, x\textsubscript3}), (\textbf{u\textsubscript2, x\textsubscript4})\} \\
-- \AUA\ = \{(\textbf{u\textsubscript3, ar\textsubscript1}), (\textbf{u\textsubscript4, ar\textsubscript2})\} \\
-- \RH\ = \{(\textbf{x\textsubscript1, x\textsubscript2}), (\textbf{x\textsubscript2, x\textsubscript3}), (\textbf{x\textsubscript3, x\textsubscript4}), (\textbf{x\textsubscript4, x\textsubscript5}), (\textbf{x\textsubscript5, x\textsubscript6})\} \\
-- \ARH\ = \{(\textbf{ar\textsubscript{1}, ar\textsubscript2})\}, \CR\ = \{\textbf{x\textsubscript{1} $\wedge$ x\textsubscript{2}}, \textbf{$\bar{\textrm{x}}$\textsubscript{1}} $\vee$ (\textbf{$\bar{\textrm{x}}$\textsubscript{2} $\wedge$ x\textsubscript{3}})\} \\
\it{can\_assign} = \{(\textbf{ar\textsubscript1}, (\textbf{x\textsubscript{1} $\wedge$ x\textsubscript{2}}), \\
\tab \stab\{\textbf{x\textsubscript4, x\textsubscript5}\}), (\textbf{ar\textsubscript1}, \textbf{$\bar{\textrm{x}}$\textsubscript{1}} $\vee$ (\textbf{$\bar{\textrm{x}}$\textsubscript{2} $\wedge$ x\textsubscript{3}}), \{\textbf{x\textsubscript6}\})\}\\
\it{can\_revoke} = \{(\textbf{ar\textsubscript1}, \{\textbf{x\textsubscript4, x\textsubscript5, x\textsubscript6}\})\}

\vspace{1ex}
\noindent
\textbf{An Equivalent AURA Instance:} \\
-- \U\ =\{\textbf{u\textsubscript1, u\textsubscript2, u\textsubscript3, u\textsubscript4}\} \\   
-- \AU\ = \{\textbf{u\textsubscript1, u\textsubscript2, u\textsubscript3, u\textsubscript4}\} \\ 
-- \OP\ = \{\textbf{assign, revoke}\} \\
-- \RN\ = \{\textbf{x\textsubscript{1}, x\textsubscript{2}, x\textsubscript3, x\textsubscript4, x\textsubscript5, x\textsubscript6}\} \\ 
-- \RNH\ = \{(\textbf{x\textsubscript1, x\textsubscript2}), (\textbf{x\textsubscript2, x\textsubscript3}), (\textbf{x\textsubscript3, x\textsubscript4}), (\textbf{x\textsubscript4, x\textsubscript5}), (\textbf{x\textsubscript5, x\textsubscript6})\} \\
-- \it{\adroles}(\textbf{u\textsubscript1}) = \{\textbf{x\textsubscript1, x\textsubscript2}\}, \it{\adroles}(\textbf{u\textsubscript2}) = \{\textbf{x\textsubscript3, x\textsubscript4}\} \\
-- \UATT\ = \{\}, \AATT\ = \{\it{aroles}\} \\
-- \scope(\it{aroles}) = \{\textbf{ar\textsubscript1, ar\textsubscript2}\}, attType(\textit{aroles}) = set, \isord(\it{aroles}) = True, \\
-- H\textsubscript{\it{aroles}} = \{(\textbf{ar\textsubscript1, ar\textsubscript2})\} \\
-- \it{aroles}(\textbf{u\textsubscript3}) = \{\textbf{ar\textsubscript1}\}, \it{aroles}(\textbf{u\textsubscript4}) = \{\textbf{ar\textsubscript2}\} \\
-- {\isauth}U\textsubscript{\textbf{assign}}(\textit{au, $\chi$, r}) $\equiv$ 
 (($\exists$\textit{ar} $\geq$ \textbf{ar\textsubscript1}). \textit{ar} $\in$ \textit{aroles}(\textit{au}) $\wedge$ 
\it{r} $\in$ \{\textbf{x\textsubscript4, x\textsubscript5}\} $\wedge$ 
(($\exists$\textit{x} $\geq$ \textbf{x\textsubscript{1}}). \it{x} $\in$ \textit{\adroles}(\textit{u}) $\wedge$ ($\exists$\textit{x} $\geq$ \textbf{x\textsubscript{2}}). \it{x} $\in$ \textit{\adroles}(\textit{u})) $\vee$ ($\exists$\textit{ar} $\geq$ \textbf{ar\textsubscript1}). \textit{ar} $\in$ \textit{aroles}(\textit{au})  $\wedge$ \it{r} $\in$ \{\textbf{x\textsubscript6}\} $\wedge$ (($\exists$\textit{x} $\geq$ \textbf{x\textsubscript{1}}). \it{x} $\notin$ \textit{\adroles}(\textit{u}) $\vee$ (($\exists$\textit{x} $\geq$ \textbf{x\textsubscript{2}}). \it{x} $\notin$ \textit{\adroles}(\textit{u}) $\wedge$ ($\exists$\textit{x} $\geq$ \textbf{x\textsubscript{3}}). \it{x} $\in$ \textit{\adroles}(\textit{u}))) 
-- {\isauth}U\textsubscript{\textbf{revoke}}(\textit{au, $\chi$, r}) $\equiv$ ($\exists$\textit{ar} $\geq$ \textbf{ar\textsubscript1}). \textit{ar} $\in$ \textit{aroles}(\textit{au}) $\wedge$ \it{r} $\in$ \{\textbf{x\textsubscript4, x\textsubscript5, x\textsubscript6}\}

\section{Mapping an Example Instance of \\Uni-ARBAC's PRA in ARPA}\label{praUniinstance}

\noindent
\textbf{An Example Uni-ARBAC's PRA Instance:}\\
\underline{Traditional RBAC Sets \& Relations:} \\
-- \U\ = \{\textbf{u\textsubscript1, u\textsubscript2, u\textsubscript3, u\textsubscript4}\} \\ 
-- \R\ = \{\textbf{r\textsubscript1, r\textsubscript2, r\textsubscript3, r\textsubscript4}\} \\
-- \P\ = \{\textbf{p\textsubscript1, p\textsubscript2, p\textsubscript3, p\textsubscript4}\} \\
-- \RH\ = \{(\textbf{r\textsubscript1, r\textsubscript2}), (\textbf{r\textsubscript2, r\textsubscript3})\}\\
\underline{Additional RBAC Sets \& Relations:} \\
-- \T\ = \{\textbf{t\textsubscript1, t\textsubscript2, t\textsubscript{3}, t\textsubscript4}\} \\
-- \tH\ = \{(\textbf{t\textsubscript1, t\textsubscript2}), (\textbf{t\textsubscript2, t\textsubscript3}), (\textbf{t\textsubscript2, t\textsubscript4})\} \\
--  \PA\ = \{(\textbf{p\textsubscript1, t\textsubscript1}), (\textbf{p\textsubscript1, t\textsubscript4}), (\textbf{p\textsubscript2, t\textsubscript4}), (\textbf{p\textsubscript4, t\textsubscript3}), (\textbf{p\textsubscript3, t\textsubscript2})\} \\
-- \TA\ = \{(\textbf{t\textsubscript1, r\textsubscript2}), (\textbf{t\textsubscript2, r\textsubscript1}), (\textbf{t\textsubscript3, r\textsubscript4}), (\textbf{t\textsubscript4, r\textsubscript3})\}\\
\underline{Derived functions} \\
-- authorized\_perms(\textbf{r\textsubscript1}) = \{\textbf{p\textsubscript3}\} \\
-- authorized\_perms(\textbf{r\textsubscript2}) = \{\textbf{p\textsubscript1}\} \\
-- authorized\_perms(\textbf{r\textsubscript3}) = \{\textbf{p\textsubscript1, p\textsubscript2}\} \\
-- authorized\_perms(\textbf{r\textsubscript4}) = \{\textbf{p\textsubscript4}\}

% \vspace{1ex}
% \noindent
% Uni-ARBAC Administrative Model Instance:\\
\noindent
\underline{Administrative Units and Partitioned Assignments} \\
-- \AU\ = \{\textbf{au\textsubscript1, au\textsubscript2}\} \\
-- \it{\adroles}(\textbf{au\textsubscript1}) = \{\textbf{r\textsubscript1, r\textsubscript2}\}, \it{\adroles}(\textbf{au\textsubscript2}) = \{\textbf{r\textsubscript3}\}, \it{tasks}(\textbf{au\textsubscript1}) = \{\textbf{t\textsubscript1, t\textsubscript2}\}, \it{tasks}(\textbf{au\textsubscript2}) = \{\textbf{t\textsubscript3, t\textsubscript4}\}\\
\underline{Derived Function} \\
-- \it{tasks}*(\textbf{au\textsubscript1}) = \{\textbf{t\textsubscript1, t\textsubscript2, t\textsubscript3, t\textsubscript4}\}, \it{tasks}*(\textbf{au\textsubscript2}) = \{\textbf{t\textsubscript3, t\textsubscript4}\} \\
\underline{Administrative User Assignments} \\
-- \it{TA\_admin} = \{(\textbf{u\textsubscript1, au\textsubscript1}), (\textbf{u\textsubscript2, au\textsubscript2})\}  \\
-- \AUH\ = \{(\textbf{au\textsubscript1, au\textsubscript2})\} \\
\underline{Task-role assignment condition in uni-ARBAC:}\\
\it{can\_manage\_task\_role}(\it{u} : \U, \it{t}: \T, \it{r}: \R) =\\
\stab ($\exists$\it{au\textsubscript{i}, au\textsubscript{j}})[(\it{u}, \it{au\textsubscript{i}}) $\in$ \it{TA\_admin} $\wedge$ 
\it{au\textsubscript{i}} $\succeq$\textsubscript{\it{au}} \it{au\textsubscript{j}} $\wedge$ \\
\stab \it{r} $\in$ \it{\adroles}(\it{au\textsubscript{j}}) $\wedge$ \it{t} $\in$ \it{tasks}*(\it{au\textsubscript{j}})]

\vspace{1ex}
\noindent
\textbf{An Equivalent ARPA instance}:\\
-- \AU\ = \{\textbf{u\textsubscript1, u\textsubscript2, u\textsubscript3, u\textsubscript4}\} \\
-- \OP\ = \{\textbf{assign, revoke}\} \\
-- \RN\ = \{\textbf{r\textsubscript1, r\textsubscript2, r\textsubscript3, r\textsubscript4}\} \\
-- \RNH\ = \{(\textbf{r\textsubscript1, r\textsubscript2}), (\textbf{r\textsubscript2, r\textsubscript3}), (\textbf{r\textsubscript3, r\textsubscript4})\} \\
-- \P\ = \{\textbf{p\textsubscript1, p\textsubscript2, p\textsubscript3, p\textsubscript4}\} \\
-- \AATT\ = \{\textit{\au, \aur}\} \\
-- \scope(\textit{\au}) =  \{\textbf{au\textsubscript1, au\textsubscript2}\}, \\
\hspace*{0.27cm}attType(\it{\au}) = set\\
-- \isord(\it{\au}) = True, \\
\hspace*{0.27cm}H\textsubscript{\it{\au}} =  \{(\textbf{au\textsubscript1, au\textsubscript2})\} \\
-- \it{\au}(\textbf{u\textsubscript1}) = \{\textbf{au\textsubscript1}\}, \it{\au}(\textbf{u\textsubscript2}) = \{\textbf{au\textsubscript2}\}, \\
\hspace*{0.27cm}\it{\au}(\textbf{u\textsubscript3}) = \{\}, \it{\au}(\textbf{u\textsubscript4}) = \{\textbf{}\} \\
-- \scope(\textit{\aur}) =  \{(\textbf{au\textsubscript1, r\textsubscript1}), \\
\hspace*{0.27cm}(\textbf{au\textsubscript1, r\textsubscript2}), (\textbf{au\textsubscript2, r\textsubscript3})\}, attType(\textit{\aur}) = set,\\
-- \isord(\it{\aur}) = False, H\textsubscript{\it{\aur}} = $\phi$ \\
-- \it{\aur}(\textbf{u\textsubscript1}) = \{(\textbf{au\textsubscript1, r\textsubscript1}), (\textbf{au\textsubscript1, r\textsubscript2}), (\textbf{au\textsubscript2, r\textsubscript3})\},\\
\hspace*{0.27cm}\it{\aur}(\textbf{u\textsubscript2}) = \{(\textbf{au\textsubscript2, r\textsubscript3})\}, \\
\vspace*{0.1cm}
\hspace*{0.2cm}\textit{\aur}(\textbf{u\textsubscript3}) = \{\}, \it{\aur}(\textbf{u\textsubscript4}) = \{\} \\
-- \PATT\ = \{\it{tasks, task\_adminu}\} \\
-- \scope(\it{tasks}) = \{\textbf{t\textsubscript1, t\textsubscript2, t\textsubscript3, t\textsubscript4}\}, attType(\it{tasks}) = set \\
-- is\_ordered(\it{tasks}) = True, H\textsubscript{\it{tasks}} = \tH\  \\
-- \it{tasks}(\textbf{p\textsubscript1}) = \{\textbf{t\textsubscript1, t\textsubscript2, t\textsubscript4}\}, \it{tasks}(\textbf{p\textsubscript2}) = \{\textbf{t\textsubscript1, t\textsubscript2, t\textsubscript4}\},\\ 
\hspace*{0.27cm}\it{tasks}(\textbf{p\textsubscript3}) = \{\textbf{t\textsubscript1, t\textsubscript2}\}, \it{tasks}(\textbf{p\textsubscript4}) = \{\textbf{t\textsubscript1, t\textsubscript2, t\textsubscript3}\} \\
-- \scope(\it{task\_adminu}) = \{(\textbf{t\textsubscript1, au\textsubscript1}), (\textbf{t\textsubscript2, au\textsubscript2})\}, \\
-- attType(\it{task\_adminu}) = set, \\
-- \isord(\it{task\_adminu}) = False, H\textsubscript{\it{task\_adminu}} = $\phi$ \\
-- \it{task\_adminu}(\textbf{p\textsubscript1}) = \{(\textbf{t\textsubscript1, au\textsubscript1}), (\textbf{t\textsubscript4, au\textsubscript2})\}, \\
 \hspace*{0.27cm}\it{\it{task\_adminu}}(\textbf{p\textsubscript2}) = \{(\textbf{t\textsubscript4, au\textsubscript2})\}, \\
\hspace*{0.27cm}\it{task\_adminu}(\textbf{p\textsubscript3}) = \{(\textbf{t\textsubscript2, au\textsubscript1})\},\\ \hspace*{0.27cm}\it{task\_adminu}(\textbf{p\textsubscript4}) = \{(\textbf{t\textsubscript3, au\textsubscript2})\} 

\vspace{1ex}
\noindent
Set of permissions $\chi$\textsubscript{\textsubscript{\it{i}}} is expressed using set-builder notation as follows:\\
%that are mapped to each task \it{t} $\in$ \T\ can be expressed as follows: \\
%\begin{enumerate}[label=(\alph*)]
$\chi$\textsubscript{\textsubscript{1}} = \{\it{p} $\vert$ \textbf{t\textsubscript1} $\in$ \it{tasks}(\it{p})\}, 
$\chi$\textsubscript{\textsubscript{2}} = \{\it{p} $\vert$ \textbf{t\textsubscript2} $\in$ \it{tasks}(\it{p})\}, \\
$\chi$\textsubscript{\textsubscript{3}} = \{\it{p} $\vert$ \textbf{t\textsubscript3} $\in$ \it{tasks}(\it{p})\}, 
$\chi$\textsubscript{\textsubscript{4}} = \{\it{p} $\vert$ \textbf{t\textsubscript4} $\in$ \it{tasks}(\it{p})\} 
%\end{enumerate}
%\vspace*{0.2ex}

\vspace{1ex}
\noindent
For each $\chi$ in \{$\chi$\textsubscript{\textsubscript{1}}, $\chi$\textsubscript{\textsubscript{2}}, $\chi$\textsubscript{\textsubscript{3}}, $\chi$\textsubscript{\textsubscript{4}}\}, authorization rule for permission-role assignment and revocation are expressed\\
\vspace{1mm}as follows:\\
%authorization rule is given below:\\ 
-- {\isauth}P\textsubscript{\textbf{assign}}(\it{u, $\chi$\textsubscript{\textsubscript{i}}, r}) $\equiv$ \\ 
$\exists$\it{au\textsubscript1,  au\textsubscript2} $\in$ \scope(\it{\au}). (\it{au\textsubscript1, au\textsubscript2}) $\in$ H\textsubscript{\it{\au}} $\wedge$
 (\it{au\textsubscript1} $\in$ \it{\au}(\it{u}) $\wedge$ (\it{au\textsubscript2, r}) $\in$  \it{\aur}(\it{u})) $\wedge$ $\exists$\it{t\textsubscript1, t\textsubscript2} $\in$ \scope(\it{tasks}). [(\it{t\textsubscript1, t\textsubscript2}) $\in$ \tH\ $\wedge$ $\forall$\it{q} $\in$ $\chi$. \it{t\textsubscript2} $\in$ \it{tasks}(\it{q}) $\wedge$ $\exists$\it{q}\q\ $\in$ (\P\ - $\chi$). \it{t\textsubscript2} $\notin$ \it{tasks}(\it{q}\q) $\wedge$ (\it{t\textsubscript2, au\textsubscript2}) 
 \vspace*{2mm} $\in$ \it{tasks\_adminu}(\it{q})]\\ 
-- {\isauth}P\textsubscript{\textbf{revoke}}(\it{u, $\chi$\textsubscript{\textsubscript{i}}, r}) $\equiv$ \\
\hspace*{4cm}{\isauth}U\textsubscript{\textbf{assign}}(\it{u, $\chi$, r})
